# Supplementary material for: Accelerating Recommender Model Training by Dynamically Skipping Stale Embeddings
Source: arXiv:2404.04270 source file (2024-03-22)
Supplement: Supplementary file 1 [file appendix.tex]

\section{Appendix}

\subsection{Mechanics of Slipstream}~\label{app:mech}
Recommendation models can mostly be decomposed into two main components. Neural network and embedding table, which store the numerical representation of all entities. Each embedding table is correlated with a categorical feature Thus, we can define a bag of $\mathbf{N}$ embeddings as:

\begin{displaymath}
{{E^{Bag}} = {E^1} \cup {E^2} \cup {E^3} \cup ... {E^N}} 
\end{displaymath}

Therefore, one single embedding table can be shown as:

\begin{displaymath}
{E^i \in \mathbb{R}^{m \times d}} 
\end{displaymath}

Where d is the hyperparameter representing the dimensionality of the embedding vector or size of each embedding entry and m is the number of embedding entries such that $\mathbf{m \gg d}$.
Each embedding entry can be written as:
\begin{displaymath}
{E_i = [ e_{i1},e_{i2}, ... , e_{id} ]}
\end{displaymath}
Each model can have multiple embedding tables and follow the form described above.

Take the embedding tables below as an example:
\begin{displaymath}
{E_1\in \mathbb{R}^{m \times d}}
\end{displaymath}
Assuming the total number of accesses during the training time is $\mathbf{M}$. Assume the number of access to each entry of $\mathbf{E_i}$ is $\mathbf{M_i}$, we can infer that  $\mathbf{M}$ is summation over discrete distribution of the random variable $\mathbf{M_i}$ over $\mathbf{i}$ or
\begin{displaymath}
{M = \sum_{i=1}^{d} {M_i}}
\end{displaymath}

We define $\mathbf{\Lambda}$ as a hyperparameter of the model to determine if an embedding entry is popular. On the same note, if embedding entry $\mathbf{E_i}$ is hot then if condition below holds
\begin{displaymath}
{\Lambda \geq {\frac{M_i}{M}}}
\end{displaymath}

These entries have the benefit of being accessed so often in comparison to other entries in the same embedding table. Hence, storing them separately can help accelerate the training.
Thus, we collect all embedding entries that follow the previous condition and call it a hot embedding table or $\mathbf{H}$. In slipstream, we store a copy of hot embedding tables on each GPU.

With respect to the definitions above, we take two snapshots of hot embedding tables at two different times $\mathbf{E_t, E_{t+1}}$. In Slipstream we choose $\mathbf{t}$ and $\mathbf{t+1}$ meticulously. These two times should be chosen in a way to captures the efficient difference magnitude. If chosen so early, the model is still getting trained and accuracy loss will be high. On the other hand, if we pick them too close to each other and closer to the end of the training, the potential speedup benefit will be jeopardized. Hence not only is it important when to take the hot embedding snapshots but also the difference between these two intervals matters as well. Therefore, we are able to depict the pattern of their change. Calculating the difference between these two, we come up with a new table $\mathbf{E_{diff}}$.

\begin{displaymath}
\mathbf{E_{diff} =  E_{t+1} - E_t} 
\end{displaymath}

\begin{displaymath}
\mathbf{E_{diff}}\in \mathbb{R}^{m \times d} 
\end{displaymath}

We set two hyperparameters $\mathbf{\alpha  \in {N}}$ and $T \in \mathbb{R}}$ for detecting staleness in embedding table entries. We consider an embedding entry as stale if and only if

\begin{displaymath}
{\alpha \geq \sum_{i=1}^{d} {\beta_i}}
\end{displaymath}

Where $\mathbf{\beta_i}$ is defined as
\begin{equation}\small
  {\beta_i} =
  \begin{cases}
    1 & \text{if  } {{E_{diff}(i)}} \geq \theta \\
    0 & \text{otherwise}
  \end{cases}
\end{equation}

Where $T$ is the threshold to determine if an element from $\mathbf{E_{diff}}$ is stale or not, and depending on the number of stale elements, we determine if the hot embedding entry is stale or not.

\subsection{Motivation for Staleness}~\label{app:change}
As a part of designing Slipstream, We needed to know if there is any point in training that results in at least some hot entries being stagnant. We picked random entries from the hot embedding table across different datasets. Considering the moving average, we notice that some hot entries do not change above a certain threshold or become stale. 

Based on Figure~\ref{fig:embeddingupdates}, across all the datasets, we observe that at a certain point during training, highly accessed or hot embedding entries are not getting updated enough with respect to the magnitude of the change. This can result in model updates that do not necessarily contribute to tangible results.  

\begin{figure*}[t]
\centering
	\includegraphics[width=1\textwidth]{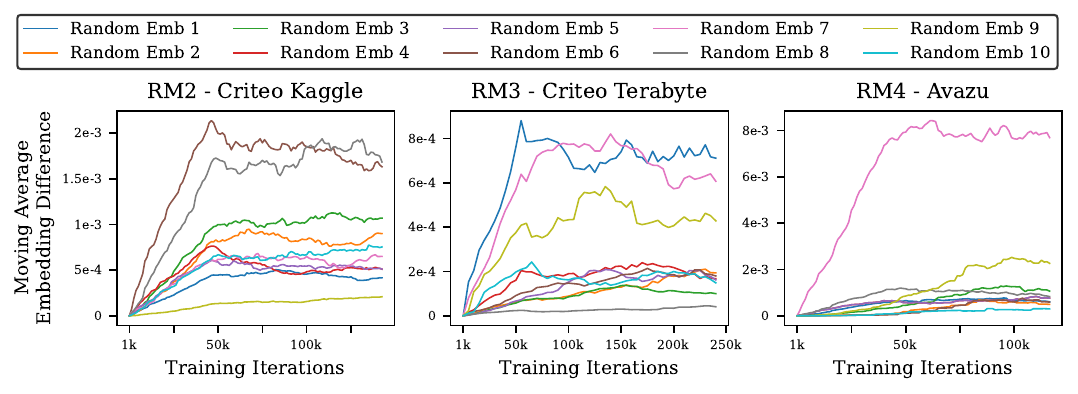}
	\caption{The difference in values over time for 10 randomly selected highly accessed popular embeddings for RM2, RM3, and RM4 recommendation models with three real-world datasets. DLRM~\cite{dlrm} is used to train these models.}
	\label{fig:embeddingupdates}
\end{figure*}
